# Supplementary material for: Double Machine Learning for Static Panel Models with Fixed Effects
Source: arXiv:2312.08174 source file (2024-12-30)
Supplement: Supplementary file 1 [file 888_additional_figs.tex]

\section{Additional Figures}\label{sec:add_figs}

%%%%%%%%%%%%%%%%%%%%%%%%%%%%%%%%%%%%%%%%%%%%%%%%%%%%%%%%%%%%%%%%%%%%%%%%%%%%%%%%%%%%%
%%%% dotplots
%%%%%%%%%%%%%%%%%%%%%%%%%%%%%%%%%%%%%%%%%%%%%%%%%%%%%%%%%%%%%%%%%%%%%%%%%%%%%%%%%%%%%
%% SHOW IN PRESENTATIONS!

% \begin{figure}[ht!]
%     \caption{Simulation results, CRE estimator}
%     \label{fig:dotplot_fd}
%     \centering
%     \subfloat{\includegraphics[scale=.8]{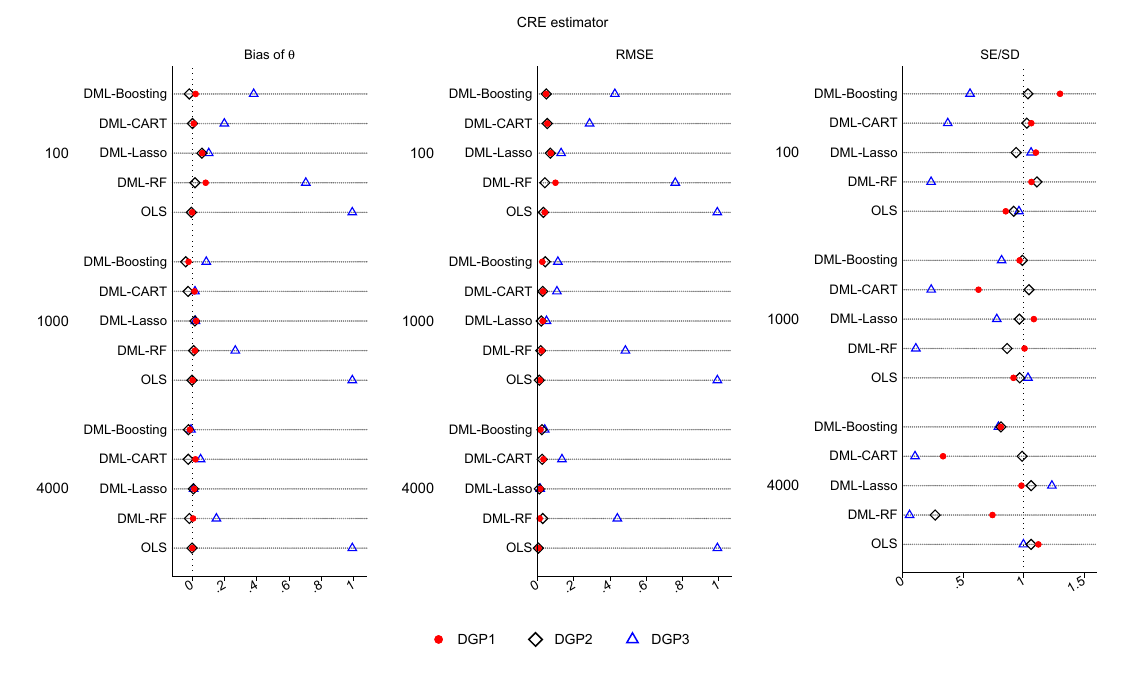}}
%     \vspace{-1mm}
%     \begin{minipage}{.9\linewidth}
%     \vspace{-1mm}
%     \emph{Note: Averages over 100 Monte Carlo replications. DGP1 is linear in the nuisance functions; DGP2 smooth non-linear; DGP3 non-smooth non-linear; time is fixed to $t=10$ time periods.}
%     \end{minipage}
% \end{figure}

% \begin{figure}[ht!]
%     \caption{Simulation results, FD estimator (with lagged inputs)}
%     \label{fig:dotplot_fd}
%     \centering
%     \subfloat{\includegraphics[scale=.8]{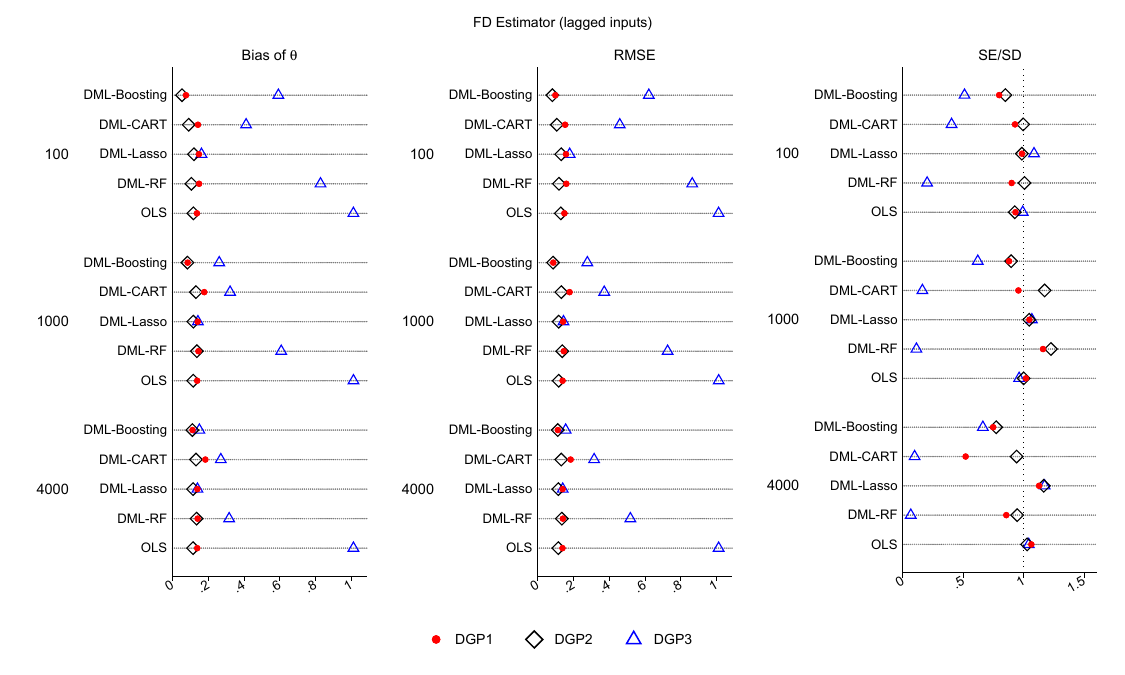}}
%     \vspace{-1mm}
%     \begin{minipage}{.9\linewidth}
%     \vspace{-1mm}
%     \emph{Note: Averages over 100 Monte Carlo replications. DGP1 is linear in the nuisance functions; DGP2 smooth non-linear; DGP3 non-smooth non-linear; time is fixed to $t=10$ time periods.}
%     \end{minipage}
% \end{figure}

%%%%%%%%%%%%%%%%%%%%%%%%%%%%%%%%%%%%%%%%%%%%%%%%%%%%%%%%%%%%%%%%%%%%%%%%%%%%%%%%%%%%%
%%%% kdensities
%%%%%%%%%%%%%%%%%%%%%%%%%%%%%%%%%%%%%%%%%%%%%%%%%%%%%%%%%%%%%%%%%%%%%%%%%%%%%%%%%%%%%
\begin{figure}[ht!]
    \centering
    \subfloat{\includegraphics[scale=.75]{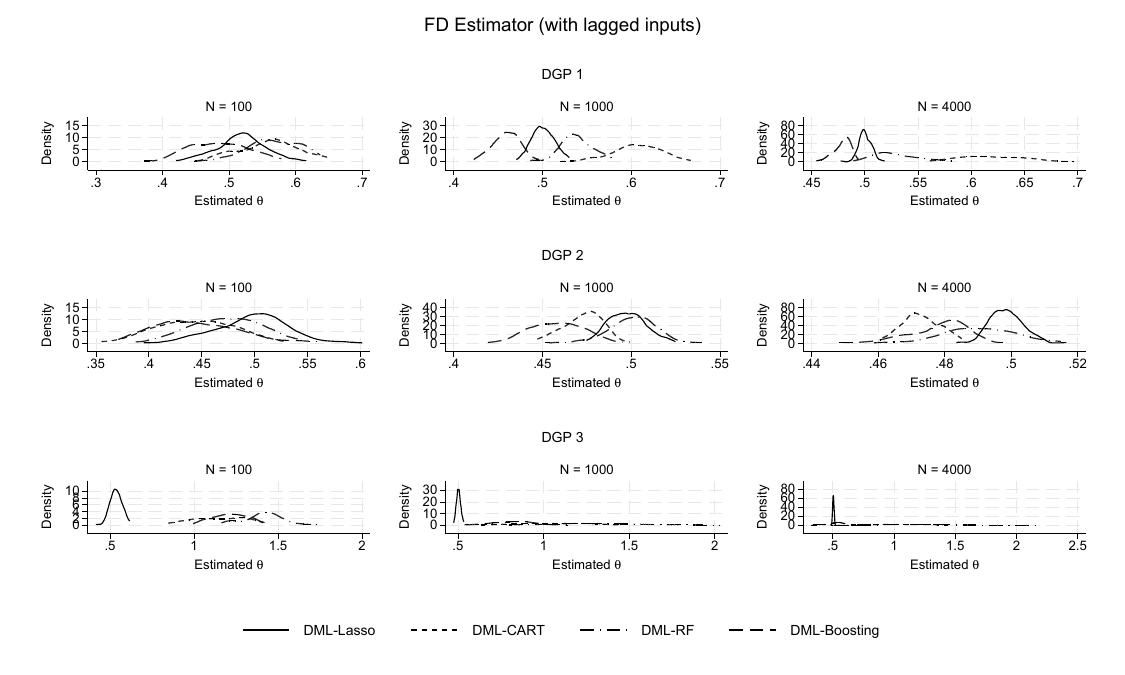}}
    \caption{Distribution of $\thetano$ across simulation designs, approximation FD estimator (with lagged inputs)}\label{fig:kdensity_dgp_fdLag}
    \vspace{1mm}
    \begin{minipage}{1\linewidth}
    \emph{Note: Comparison of estimated target parameter in 100 Monte Carlo replications. The true target parameter $\theta$ is 0.50. The sample size is fixed to 1000 cross-sectional units and 10 time periods. Hyperparameters of base learners are tuned via grid search.}
    \end{minipage}
\end{figure}

\begin{figure}[ht!]
    \centering
    \subfloat{\includegraphics[scale=.75]{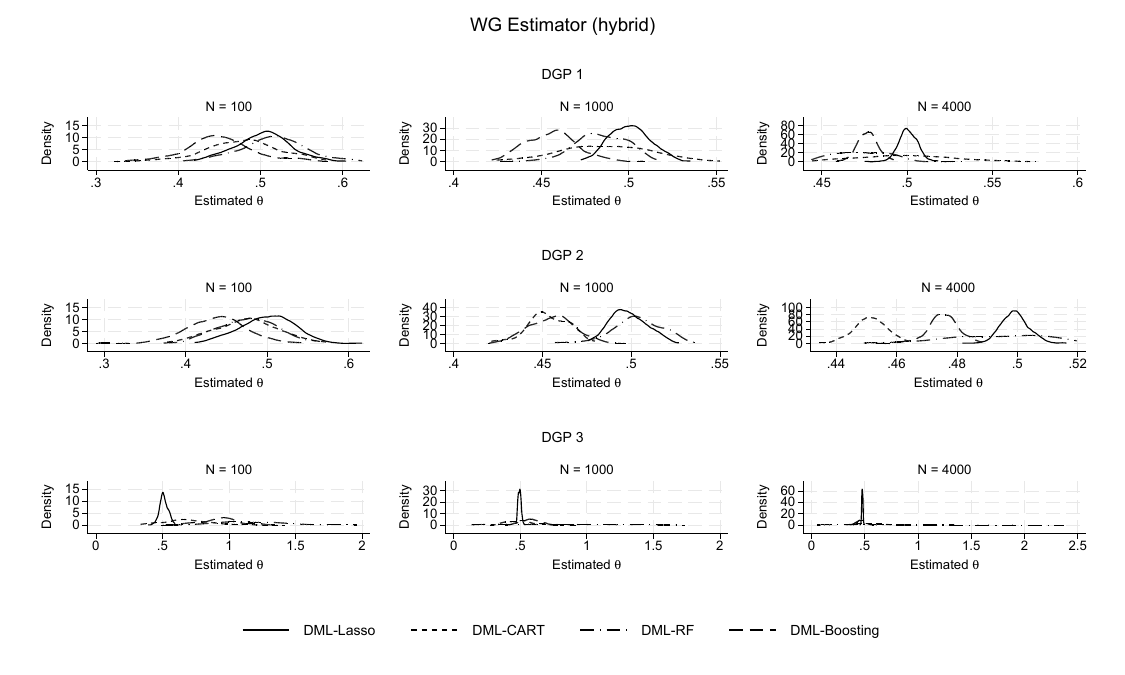}}
    \caption{Distribution of $\thetano$ across simulation designs, WG estimator (hybrid)}\label{fig:kdensity_dgp_wg} 
    \vspace{1mm}
    \begin{minipage}{1\linewidth}
    \emph{Note: Comparison of estimated target parameter in 100 Monte Carlo replications. The true target parameter $\theta$ is 0.50. The sample size is fixed to 1000 cross-sectional units and 10 time periods. Hyperparameters of base learners are tuned via grid search.}
    \end{minipage}
\end{figure}
