# Supplementary material for: Double Machine Learning for Static Panel Models with Fixed Effects
Source: arXiv:2312.08174 source file (2024-12-30)
Supplement: Supplementary file 2 [file SI_derivation_plrp.tex]

%%%%%%%%%%%%%%%%%%%%%%%%%%%%%%%%%%%%%%%%%%%%%%%%%%%%%%%%%%%%%%%%%%%%%%%%%%%%%%%%
\section{Derivation of the Partially Linear Panel Regression Model}\label{sec:appx_model}
\setcounter{equation}{0}
%%%%%%%%%%%%%%%%%%%%%%%%%%%%%%%%%%%%%%%%%%%%%%%%%%%%%%%%%%%%%%%%%%%%%%%%%%%%%%%%
We now describe the assumptions the unknown data generating process (DGP) must satisfy for the DML estimation procedures we propositionose in the next section to have a causal interpretation and consistent and asymptotically normal estimators.

First, suppose the panel study collects information on each of $N$ individuals at each of the $T$ time periods, or waves. % where $N\gg T$ for standard asymptotic theory to apply. 
To simplify notation, we assume a balanced panel with observed data on every individual at all $T$ waves.% such that $T_i=T_j=T$ for $i\ne j$.
\footnote{The estimation problem and results hold with unbalanced panel with appropositionriate modifications in the notation.} %The total number of panel data units is $NT=n$.  
Let $\{\yit,\dit,\xit : \ t=1,\ldots,T\}$ be independent and identically distributed (\emph{iid}) random variables for individuals \mbox{$i=1,\ldots,N$}, where $\yit$ is the outcome (or dependent) variable, $\dit$ a continuous or binary treatment  variable (or intervention), and $\xit$ a $p\times 1$ vector of regressors, usually including a constant term, included to capture time-varying confounding induced by non-random treatment selection. 
For continuous $\dit$, if $\dit\geq 0$ we presume a dose-response relationship with $\dit=0$ indicating null treatment; otherwise, $\dit$ is taken to be centered around its mean $\mu_D$ such that $\dit \equiv \dit-\mu_D$. For binary $\dit\in\{0,1\}$, $\dit=0$ is taken to indicate the absence and $\dit=1$ the presence of treatment.
%We allow the dimension of $\xit$ $p$ to be large but smaller than $N$ such that $p/N\to 0$, \red{and only a small subset of them are relevant in determining the effect of the treatmentment $s<p$ and $s\ll N$ (\emph{sparsity.})} %Too early to introduce this

%%%%%%%%%%%%%%%%%%%%%%%%%%%%%%%%%%%%%%%%%%%%%%%%%%%%%%%%%%%%%%%%%%%%%%%%%%%%%%%%
Second, we derive a partially linear model \citep{robinson1988} for panel data by using the potential outcomes causal framework \citep{rubin1974}. This allows estimation to proceed without relying on tightly specified parametric model for the DGP, only a reduced-form model parameterized directly in terms of the target effect \citep{lechner2015}. This begins by defining $\yit(.)=\{y_{it}(d):d\in \Omega_D\}$ as the set of potential outcomes for individual $i$ at wave $t$, where $\yit(d)$ is the realization of the outcome for individual $i$ at wave $t$ were the treatment level to be set to $d$, with one potential outcome for every possible value the treatment could take. The realizations of the wave $t$ potential outcomes are taken to occur before treatment selection at wave $t$, and are linked to the observed outcome by the {\em consistency assumption} that $y_{it}(d_{it})=y_{it}$ is the observed potential outcome with the others latent {\em counterfactuals}.\footnote{The stable unit treatment value (SUTVA) assumption, that $y_{it}(d)$ does not depend on the treatment assignments of any other individual, is implicitly taken to hold.} In the interval preceding wave $t$, it is also presumed that the realization of time-varying predictor $\xit$ precedes that of $(y_{it},d_{it})$.

Then define the set $\xi_i$ of %individual-level heterogeneity terms $\alpha_i$ and $\gamma_i$ to represent the combined effects of
omitted time-invariant variables influencing $(\yit,\dit)$, and the set $L_{t-1}(w_i) = \{w_{i1},...,w_{it-1}\}$ to represent the lags of variable(s) $w$ available at wave $t$ such that $L_0(w_i)\equiv\varnothing$. Using this notation, the first assumptions which must be satisfied by the causal data generating process can be expressed as follows:
%where the  parmeter of interest, on which we want to conduct inference, is the average treatment effect (ATE) defined as \mbox{$\theta_0  \equiv \E[\yit(d)-\yit(0)]$}.  For identification of ATE the following standard assumptions hold
\begin{enumerate}[label=\sc{Assumption }{\thesection.\arabic*}, leftmargin=3.5cm]
    \item \emph{(No feedback to predictors)} $\xit \indep{}  {L_{t-1}(y_i,d_i)}   L_{t-1}({\bf x}_i),\xi_i.$  \label{item:asm_feedback}
    \item \emph{(Static panel)} $\yit,\dit  \indep{}  {L_{t-1}(y_i,{\bf x}_i,d_i)} \xit,\xi_i$. \label{item:asm_nolags}
\end{enumerate}
\vspace{-0.05cm}
\noindent \ref{item:asm_feedback} precludes the outcome and treatment lags from having any direct causal effect, or any indirect effect mediated by omitted variables, on the process generating the time-varying predictors at wave $t$, once the history of the time-varying predictors and the individual-heterogeneity term have been conditioned on.  \ref{item:asm_nolags} is that $\xi_i$ together with $\xit$ explain all lag-dependence of $(\yit,\dit)$. This assumption is plausible if the data generating process involves no causal effect of $L_{t-1}(y_i,d_i,{\bf x}_i)$ on $(\yit,\dit)$ so that any lag dependence is due to non-causal autocorrelation. This static panel assumption, if plausible for the application to hand, avoids the {\em initial conditions problem} which would arise were the panel study to have started after the joint process began. Extending the estimators presented below to allow for first-order lag-dependence is discussed in Section~\ref{sec:conclusion}.

\ref{item:asm_feedback} and \ref{item:asm_nolags} together ensure that the joint distribution of outcomes and treatments given the time-varying predictors and omitted time-invariant influences satisfies
\[
p\{y_{i1},d_{i1},...,y_{iT},d_{iT}|L_T({\bf x}_i),\xi_i\}=\prod_{t=1}^Tp(y_{it},d_{it}|\xit,\xi_i),
\]
where $p$ denotes a density function for the (conditional or joint) distribution indicated by its arguments. It is thus unnecessary to model the distribution of the time-varying predictors. %assumes that a unit cannot receive multiple treatments and rules out spill-over effects and general equilibrium effects.
%\ref{item:asm_selection_fe}  (also knows as \emph{unconfoundedness} or \emph{ignorable selection}) states that conditional on all the explanatory variables and unobserved effects, treatment assignment is independent of the distribution of potential outcomes. In other words, it means that there are no other possible variables that jointly affect both the treatment and potential outcome (i.e., confounders). %It implies that treated and controlled units can be matched such that the latter can be used as counterfactual for the former.

The causal effect can be identified provided that the following condition holds:
\begin{enumerate}[label=\sc{Assumption }{\thesection.\arabic*},  leftmargin=3.5cm]
\setcounter{enumi}{2}
    \item \emph{(Selection on observables and omitted time-invariant variables)}\\ $\yit(.)\indep{}\dit \xit,\xi_i$.  \label{item:asm_selection_fe} 
    \item \emph{(Homogeneity of the treatment effect)} 
    $\E\{\yit(d)-\yit(0)|\xit,\xi_i\}=d\theta_0$. \label{item:asm_effect_fe}   
\end{enumerate}
\noindent \ref{item:asm_selection_fe} states that treatment selection at wave $t$ is ignorable given $\xit$ and latent $\xi_i$. \ref{item:asm_effect_fe} means that the average effect of treatment-level $d$ is homogeneous (i.e., mean-independent of $\xit$ and $\xi_i$), which holds if $y_{it}(d)-y_{it}(0)$ is constant or varies randomly between individuals; for non-binary treatments, this assumption additionally implies a linear dose-response relationship because the mean of $\yit(d)-\yit(0)$ is linear in $d$. Note that it is possible to relax this assumption and estimate non-linear heterogeneous treatment effects (i.e., when the average treatment effect depends on $\xit$) in what follows (see propositionosition \ref{prop:neyman} and Theorem \ref{thm:cre_dml}), but we will focus on the homogeneous case.\footnote{Heterogeneous causal effects can be estimated if the analyst is prepared to specify parametric model $E[\yit(d)-\yit(0) |\xit,\xi_i]=f_{\btheta_0}(d;\xit,t)$. In fact, the analyst is specifying the marginal model $f_{\theta_0}\equiv E[{\tilde f}_{\theta_0}\mid\xit]$, which applies to all populations if heterogeneity is mean-independent of $\xi_i$ under the DGP, but is otherwise only relevant for populations with the same distribution of $\xi_i$ (the CRE and transformation approaches below are both marginal).}
%[MODEL NOT INTRODUCED YET] A PO-PLR would also require evaluating $\vit=f_{\btheta_0}(\dit;\xit,t) -E\{f_{\btheta_0}(\dit;\xit,t)|\xit,\alpha_i\}$, but this would be based on the same treatment equation residual in (\ref{eqn:plr2_v}) were $f$ curvilinear or otherwise such that $\E\{f_{\btheta_0}(\dit;\xit,t)|\xit,\alpha_i\}=f_{\btheta_0}\{m_0(\xit,\alpha_i);\xit,t\}$.}
%%%%%%%%%%%%%%%%%%%%%%%%%%%%%%%%%%%%%%%%%%%%

To derive the static panel data model with unobserved individual heterogeneity, we note that \ref{item:asm_selection_fe} automatically leads to {\em conditional mean independence}
\[
E[y_{it}(0)|\dit,\xit,\xi_i\}=E[y_{it}(0)|\xit,\xi_i]=E[E[y_{it}(0)|\dit,\xit,\xi_i]|\xit,\xi_i],
\]
with the final equality following from iterated expectations. Further, under \ref{item:asm_selection_fe}  and \ref{item:asm_effect_fe}, $E[\yit - y_{it}(0)|\dit,\xit,\xi_i]=\dit\theta_0$ or $E[y_{it}(0)|\dit,\xit,\xi_i]=E[\yit|\dit,\xit,\xi_i] - \dit\theta_0$, and so it follows from conditional mean independence that
\begin{equation*} 
E[\yit|\dit,\xit,\xi_i] -\dit\theta_0 = E[\yit|\xit,\xi_i]-E[\dit|\xit,\xi_i]\theta_0,
\end{equation*}

\noindent which implies the reduced-form model
\begin{equation}
\label{eqn:plriv_y}
\yit = d_{it}\theta_0  + g_0(\xit,\xi_i) +  \uit,
\end{equation}
where $g_0(\xit,\xi_i)=E[y_{it}(0)|\xit,\xi_i]$ and, by construction, $E[u_{it}|d_{it},\xit,\xi_i]=0$.  Under the same conditional mean independence assumption as above, the partialling-out (PO) approach is an the alternative parameterization of the same model as
\begin{equation}
\label{eqn:plr_y}
\yit = v_{it}\theta_0  + l_0(\xit,\xi_i) +  \uit,
\end{equation}
where $l_0(\xit,\xi_i)=E[y_{it}|\xit,\xi_i]$, $E[u_{it}| v_{it},\xit,\xi_i]=0$,
\begin{equation}
\label{eqn:plr_v}
\vit = \dit - m_0(\xit,\xi_i),
\end{equation}
and $m_0(\xit,\xi_i)=E[\dit|\xit,\xi_i]$ implies that $E[v_{it}| \xit,\xi_i]=0$. The advantage of the second parameterization, to be exploited further on, is that $l_0$ is the mean of the observed $\yit$ rather than (partially) counterfactual $y_{it}(0)$.  

The presence of latent $\xi_i$ means that neither model (\ref{eqn:plriv_y}) nor (\ref{eqn:plr_y})-(\ref{eqn:plr_v}) can feasibly be estimated without the following further assumption:
\begin{enumerate}[label=\sc{Assumption }{\thesection.\arabic*}, leftmargin=3.5cm]
\setcounter{enumi}{4}
    \item \emph{(Separability)} %
    $l_0(\xit,\xi_i)=l_1(\xit)+\alpha_i$ and $m_0(\xit,\xi_i) = m_1(\xit)+\gamma_i$.  \label{item:asm_additive}
\end{enumerate}
\noindent  %, and will generally be be correlated with moments $\E(\alpha_i)=\E(\gamma_i)=0$ and $E(\alpha_i\gamma_i)\neq 0$. 

%\mbox{\ref{item:asm_additive}} 
\noindent This assumption allows us to rewrite model (\ref{eqn:plriv_y}) as the partially linear panel regression (PLPR) model
\begin{equation}
 \yit = \dit\theta_0 + g_1(\xit) + \alpha_i + \uit,
\end{equation}
because it also follows that $g_0(\xit,\xi)=g_1(\xit)+\alpha_i$. Moreover, from~\mbox{(\ref{eqn:plr_y})-(\ref{eqn:plr_v})}, the partialled-out partially linear panel regression (PO-PLPR) is
\begin{align}
& \yit = \vit\theta_0  + l_1(\xit) + \alpha_i + \uit, \label{eqn:plr2_y} \\
& \vit = \dit - m_1(\xit) - \gamma_i \label{eqn:plr2_v}.
\end{align}
Both models are extensions of \citet{robinson1988}'s PLR model to panel data with fixed effects, where $\alpha_i$ and $\gamma_i$ are generally correlated because both are some unknown functions of the omitted time-invariant influences~$\xi_i$.
