# Supplementary material for: Double Machine Learning for Static Panel Models with Fixed Effects
Source: arXiv:2312.08174 source file (2024-12-30)
Supplement: Supplementary file 3 [file appendix.tex]

%%%%NO
\subsection{Non-orthogonal scores}
The non-orthogonal (NO) score function for $\theta$  
\begin{equation}\label{eqn:nsf_theta}
\normalsize
 \psi^{no}(W; \theta, \eta) =  - \big(\Dii'\Dii)\theta + \Dii'\big(\Yii-\Xii\bhat\big) 
 %- \tdit^2\theta + \tdit\big(\tyit- \widehat{l}(\txit)\big)
\end{equation}

The estimator of the causal parameter is derived as 
\begin{align}\label{eqn:theta}
\normalsize
 &\E\big[\psi^{no}(W; \theta, \eta)\big] = 0\\
 & \thetano=\Bigg(\frac{1}{N}\sum_{i=1}^N \Dii'\Dii \Bigg)\inv \frac{1}{N}\sum_{i=1}^N  \Dii'(\Yii-\Xii\bhat)
\end{align}

Note that the regularisation bias of the NO score arises from selection using only the output equation (not in line with  the Frisch-Waugh theorem) and because the parameters converge to zero at a slower rate.

The non-orthogonal IV-type (NO-IV) score function for $\theta$  
\begin{equation}\label{eqn:nsf_theta}
\normalsize
 \psi^{no-iv}(W; \theta, \eta) =  - \big(\Dii'\Dii\big)\theta + \Dii'\big(\Yii-\Xii\bhat\big) 
\end{equation}

The estimator of the causal parameter is derived as 
\begin{align}\label{eqn:theta}
\normalsize
 &\E\big[\psi^{no-iv}(W; \theta, \eta)\big] = 0\\
 & \thetano=\Bigg(\frac{1}{N}\sum_{i=1}^N \Dii'\Dii \Bigg)\inv \frac{1}{N}\sum_{i=1}^N  \Dii'(\Yii-\Xii\bhat)
\end{align}

\subsection{OLS and non-orthogonal score}
\begin{equation}
    \bhat = \underset{\bbeta\in\R^p}{\argmin}\bb\Yii-\Xii\bbeta\bb^2_2
\end{equation}
\noidnent Note that we are ignoring Equation~\eqref{eqn:treat} which makes $\bhat$ biased due to OVB.
%%convergence in prob of beta_hat
\begin{align}
    N(\bhat-\bbeta)&= \Bigg(\frac{1}{N}\sum_i\Xii'\Xii\Bigg)\inv\frac{1}{N}\sum_i\Xii'(\Dii\theta+\tui)\\
    & = \Bigg(\frac{1}{N}\sum_i\Xii'\Xii\Bigg)\inv \frac{1}{N}\sum_i\Xii'\Dii\theta+ \Bigg(\frac{1}{N}\sum_i\Xii'\Xii\Bigg)\inv\frac{1}{N}\sum_i\Xii'\tui\\
    &\overset{p}{\to} \Cx\inv\Cx\dnot\theta \notag\\
    &=\dnot\theta\ne \zero_p
\end{align}
\red{[LASSO] $\|\bhat-\bbeta\|_1 \lesssim s\sqrt{\log P/N} $}
%% N\inv\sum_i D_i'D_i
\begin{align}
\frac{1}{N}\sum_i\Dii'\Dii & = \frac{1}{N}\sum_i \|\Xii+\tvi\dhat \|^2_2\\
& = \frac{1}{N}\sum_i\dhat'\Xii'\Xii \dhat + \frac{2}{N}\dhat'\sum_i\Xii'\Vii + \frac{1}{N}\sum_i\tvi'\tvi\\
&\overset{p}{\to}\dnot'\Cx\dnot+ \sigma^2_v \equiv \Cd < \infty
\end{align}

%% N\inv\sum_i D_i'X_i
\begin{align}
\frac{1}{N}\sum_i\Dii'\Xii & = \frac{1}{N}\sum_i \Big(\Xii\dhat+\tvi\Big)' \Xii\\
& = \dhat'\frac{1}{N}\sum_i\Xii'\Xii  + \frac{1}{N}\sum_i\tvi'\Xii\\
&\overset{p}{\to}\dnot'\Cx \equiv \Cdx < \infty
\end{align}
\noindent it is never equal to zero if there is at least a coefficient that is non-zero. Note that $N\inv\sum_i\Xii'\Dii\overset{p}{\to}\Cx'\dnot$

\begin{align}
    N(\thetano-\theta)&= -\Bigg(\frac{1}{N}\sum_i\Dii'\Dii\Bigg)\inv\frac{1}{N}\sum_i\Dii'\Xii(\bhat-\bbeta)\\
    & +\Bigg(\frac{1}{N}\sum_i\Dii'\Dii\Bigg)\inv\frac{1}{N}\sum_i\Dii'\tui\\
    &\overset{p}{\to} - (\dnot'\Cx\dnot+\sigma^2_v)\inv\dnot'\Cx\dnot\theta\\
    & = - \bigg(\frac{\dnot'\Cx\dnot}{\dnot'\Cx\dnot+\sigma^2_v}\bigg)\,\theta \\
    & = -\phi\theta<0 \notag
\end{align}
\noindent The quantities are all positive, so the estimator of the causal parameter is always downward biased. If $\sigma^2_v=0$ the estimator is consistent and unbiased but this is not the case ($\uparrow \sigma^2_v \Rightarrow\downarrow \phi\Rightarrow \thetano$ reducing the bias). \red{Is $\phi\in(0,1)$ or $\phi>1$?} Therefore,
\begin{equation}
N\thetano \overset{p}{\to} \theta(1-\phi)
\end{equation}
The bias arises due to omitted variable bias (OVB) by ignoring the treatment equation. 

The OVB \red{lower} bound is characterized by magnitude of the coefficients corresponding to the \red{non-zero} components of the parameters in Equations~\eqref{eqn:out}-\eqref{eqn:treat}. \red{With LASSO, the regularisation bias is a form of OVB because the variable selection is done by using the output equation only (But why is the bias lower than OLS?).  See \citet{wuthrich2021} for OVB in LASSO. They find that large OVBs are persistent across a range of empirically relevant settings and can occur even
when $n$ is large and larger than $p$, and the sparsity parameter $k$ is small. They document that the magnitude of the biases varies substantially depending on the regularization choice. [To paraphrase but this is our case!]}

\subsection{OLS and orthogonal score}
\begin{equation}
    \dhat = \underset{\bdelta\in\R^p}{\argmin}\bb\Dii-\Xii\bdelta\bb^2_2
\end{equation}

\begin{align}
    N(\dhat-\bdelta)&= \Bigg(\frac{1}{N}\sum_i\Xii'\Xii\Bigg)\inv\frac{1}{N}\sum_i\Xii'\tvi\\
    &\overset{p}{\to} \zero
\end{align}
\noindent under strong exogeneity.
%% N\inv\sum_i V_i'V_i
\begin{align}
\frac{1}{N}\sum_i\Vii'\Vii & = \frac{1}{N}\sum_i \|\Dii+\Xii\dhat \|^2_2\notag\\
& = \frac{1}{N}\sum_i\Dii'\Dii - \frac{2}{N}\dhat'\sum_i\Xii'\Dii + \frac{1}{N}\sum_i\dhat'\Xii'\Xii\dhat\\
&\overset{p}{\to}\dnot'\Cx\dnot+ \sigma^2_v -2\dnot'\Cx\dnot+\dnot'\Cx\dnot\notag\\
&=\sigma^2_v>0
\end{align}

\begin{align}
\thetaor & =\Bigg(\frac{1}{N}\sum_{i=1}^N \Vii'\Vii \Bigg)\inv \frac{1}{N}\sum_{i=1}^N  \Vii'\big(\Yii-\Xii\bhat \big)\\\
 & =\Bigg(\frac{1}{N}\sum_{i=1}^N \Vii'\Vii \Bigg)\inv \Bigg\{\frac{1}{N}\sum_{i=1}^N \big(\Dii-\Xii\dhat\big)'\big(\Dii\theta+\Xii\big(\bbeta-\bhat\big)\big)+\tui\Bigg\} \notag\\
 & =\Bigg(\frac{1}{N}\sum_{i=1}^N \Vii'\Vii \Bigg)\inv \Bigg\{\frac{1}{N}\sum_{i=1}^N \Big(\Dii'\Dii\theta-\Dii'\Xii\big(\bhat-\bbeta\big)+\Dii'\tui-\dhat'\Xii'\Di\theta+\dhat'\Xii'\Xii\big(\bhat-\bbeta\big)-\dhat'\Xii'\tui \Big)\Bigg\}\notag\\
 &\overset{p}{\to}(\sigma^2_v)\inv\Big\{(\dnot'\Cx\dnot+\sigma^2_v)\theta-\dnot'\Cx\dnot\theta-\dnot'\Cx\dnot\theta+\dnot'\Cx\dnot\theta\Big\}\\
 & =\theta\notag
 \end{align}
