# Supplementary material for: Double Machine Learning for Static Panel Models with Fixed Effects
Source: arXiv:2312.08174 source file (2024-12-30)
Supplement: Supplementary file 5 [file SI_dml_algorithm.tex]

\section{DML Algorithm for Panel Data}\label{sec:dml_algorithm}
This section describes the algorithm relative to the DML method for panel data to estimate the target (or causal) parameter of interest. The algorithm follows the main steps of Algorithm~2 in \citet{chernozhukov2018} but adapts it to the panel data framework when also the time dimension is present. 

\begin{algorithm}[\textsc{DML estimator}] 
\textnormal{Let $\bmeta$ be the nuisance parameters to learn, $\theta$ the target parameter to estimate, $p$ the number of confounding variables in the model, and $N$ the number of cross-sectional units observed in the sample for up to $T$ time periods (or waves).}
\begin{center}
\begin{list}
{\textsc{Step} \arabic{bean}.}{\usecounter{bean}}
    \item  \textnormal{\textsc{(Sample splitting and cross-fitting)} Randomly partition the cross-sectional units in the estimating sample into $k$ folds of the same size. Denote the units in fold \mbox{$k=1,\ldots,K$} by $\Wk\subset\mathcal{W}$ and let $\Wk^c$ be its complement such that $N_k\equiv |\Wk| = N/K$, $|\Wk^c|=N-N_k$ and, because the folds are mutually exclusive and exhaustive, $\Wk\cap\mathcal{W}_j=\Wk\cap\Wk^c=\varnothing$ and $\Wk\cup\Wk^c=\mathcal{W}_1\cup\ldots\cup\mathcal{W}_K=\mathcal{W}$. For \mbox{$K>2$}, the larger complementary sample $\Wk^c$ is used to learn the potentially complex nuisance parameters $\bmeta$, and $\Wk$ for the relatively simple task of estimating the target parameter $\theta_0$. Because each unit $i$ and its whole time series is assigned to the same fold, the algorithm performs a \emph{k-fold block} cross-fitting.  Sample splitting with cross-fitting (when $K\ge2$ and the folds swap roles) reduces the overfitting bias and restores efficiency.}
    
    \vspace{2mm}
 
    \item  \textnormal{\textsc{(Nuisance learning)} Learning the vector of nuisance parameters $\bmeta$ from the data of the units in the complementary sample $\Wk^c$ using one of the approaches from Section~\ref{sec:nuisance}. The learned prediction rule, denoted by $\widehat{\bmeta}_k$, is used to construct the Neyman orthogonal score function $\bmpsi^\perp_k(W; \theta, \widehat{\bmeta}_k)$ for each fold.}\\

    \vspace{2mm}

    \item  \textnormal{\textsc{(Estimation)}  The DML estimator $\widehat{\theta}$ for the $k$-th fold is derived in the second stage by solving %the finite-sample analog of the moment condition~\eqref{eqn:mom_cond} with respect to $\theta$
    \begin{equation}\label{eqn:fmom_cond}
    \frac{1}{N_k}\sum_{i\in \Wk} \bmpsi^\perp_k(W_i; \theta, \widehat{\bmeta}_k)  = \zero,
    \end{equation}
    \noindent with respect to $\theta$ using data from the estimation sample $\Wk$, and has closed-form solution model
      \begin{equation}
       \thetano_k = \Bigg(\frac{1}{N_k}\sum_{i\in\Wk}\hvi'\hvi \Bigg)\inv %
       \frac{1}{N_k}\sum_{i\in\Wk} \hvi'\hui.
      \end{equation}
    \noindent  where $\hvi = (\widehat{v}_{i1},\dots,\widehat{v}_{iT})'$ and $\hui = (\widehat{u}_{i1},\dots,\widehat{u}_{iT})'$.\footnote{The DML estimator for the IV-PLR model is $\thetano_k = \Big(\frac{1}{N_k}\sum_{i\in\Wk} \di'\hvi \Big)\inv \frac{1}{N_k}\sum_{i\in\Wk}\di'\hui$.} 
    The final estimated target parameter $\thetano$ is the average over the $k$ folds. Without loss of generality, we set $\Sigma_0 = \I_T$ in equation~\eqref{eqn:sec_score} and not estimate it. The heteroskedastic variance for $\hat{\theta}$ in fold $k$
    \begin{equation}
        \widehat{\sigma}^2_k = \widehat{J}_k\inv\Bigg\{\frac{1}{N_k}\sum_{i\in \Wk}\psi^\perp({W}_i; \theta, \widehat{\bf{\bmeta}}_{k})\psi^\perp(W_i; \theta, \widehat{\bmeta}_{k})'\Bigg\} \widehat{J}_k\inv
    \end{equation}
    \noindent where $\widehat{J}_k =N_k\inv\sum_{i\in \Wk}\hvi'\hvi$, and $\psi^\perp(W_{i}; \theta, \widehat{\bmeta}_{k})'$ is the transpose of $\psi^\perp(W_{i}; \theta, \widehat{\bmeta}_{k})$. The final variance of the target parameter, $\widehat{\sigma}^2$, is the average variance across the $k$-folds plus a finite-sample correction, $(\thetano_k-K\inv\sum_k\thetano_k)^2$, weighted by the number of units in the cluster to account for the variation introduced by sampling splitting \citep[p.~C30]{chernozhukov2018}. }\\

    \vspace{2mm}

    \item \textnormal{\textsc{(Iteration)} Repeat \textsc{Steps}~1-3 for each of the $k$-folds and average out the results.}
\end{list}
\end{center}
\end{algorithm}
